# Supplementary material for: Sensor-Space Based Robust Kinematic Control of Redundant Soft Manipulator by Learning
Source: arXiv:2507.16842 source file (2025-07-19)
Supplement: Supplementary file 1 [file Appendix.tex]

%\section*{Appendix: SVD for Computing the Rotation Matrix}

%$\mathbf{R}$ can be obtained ...
